# Supplementary material for: Charge density waves in disordered media circumventing the Imry-Ma argument
Source: arXiv:1601.03041 ancillary file (2016-01-12)
Supplement: Supplementary file 1 [file supplemental_information_imry_ma.pdf]

# Supplemental Information: Charge density waves in disordered media circumventing the Imry-Ma argument

Hitesh J. Changlani,[1] Norm M. Tubman,[2,1] and Taylor L. Hughes[1]

[1]Department of Physics, University of Illinois at Urbana-Champaign, Urbana, Illinois 61801, USA
[2]Department of Chemistry, University of California, Berkeley, California 94720, USA
(Dated: January 10, 2016)

## I. NUMERICAL METHODS

In this section, we discuss details of our simulations performed with the density matrix renormalization group (DMRG) [1] algorithm. The DMRG technique is based on the idea that a many-body wavefunction can be written as a matrix product state (MPS) whose parameters (elements of the matrices) can be efficiently optimized. The accuracy of the MPS representation for describing the exact state is dependent on the dimension of the matrices ($m$). While any wavefunction is exactly representable as an MPS in the $m \to \infty$ limit, the utility of the DMRG technique/MPS decomposition is apparent when $m$ is small (typically few hundred to few thousand). This is especially true for low energy states of gapped one dimensional systems with short range hoppings and interactions, with open or pinned boundary conditions. The DMRG calculations in this paper were performed with a combination of our codes and the open-source ITensor software [2] and the Algorithms and Libraries for Physics Simulations (ALPS) [3] library.

### A. Simulation strategy

We work with spinless electrons at half filling on chains with an even number of sites. At zero disorder and large $V/t$, for a chain with open boundary conditions, it is favorable for charge density wave (CDW) order to propagate from both ends. These CDW orders emerge from opposite sublattices and hence interfere in the bulk of the chain; such a superposition of states restores translational invariance. While the existence of the underlying CDW order can still be detected in the bulk from density-density correlations, it is easier (and computationally more efficient) to explicitly break the symmetry between the two orders. This allows us to access the (CDW) order directly by simply measuring electron density at every site.

To break the sublattice symmetry, we apply a pinning field in all cases (with or without disorder) to the left-most site, by using an on-site energy of $\epsilon = 20t$ at that site. No pinning field is applied at the right end. This suppresses the electron occupation at the left-most site to a low value and ensures that the CDW emerging from the left boundary is in phase with the CDW that naturally emerges from the right boundary. This choice of boundary conditions induces only a small bias towards a stable CDW. This is verified in our findings showing that the random monomer and trimer models do not have stable CDW phases even when the disorder is small, and that the random dimer and quadrumer models transition into the disordered phase at a sufficiently large interaction dependent disorder strength.

Such symmetry breaking strategies also reduce the entanglement of the ground state quantum many-body wavefunction, allowing for smaller bond dimensions to be used in the DMRG algorithm. For our calculations a bond dimension of $m = 300 - 500$ was used, which yielded truncation errors of the order of $10^{-14}$ to $10^{-8}$, with variations for different realizations and disorder and interaction strengths.

### B. Disorder-averaging and finite size effects

We presented results for disorder-averaged domain sizes as a function of the disorder strength (Fig. 4 of the main text), using about 80 realizations each of length 1000 sites. A "domain" was defined as a region where local CDW (on either sublattice) was present. This was identified by monitoring "domain walls" - regions where the (dominant) occupation of the electrons changed from one sublattice to the other. This was practically done by going along the chain and identifying regions where the electronic occupation of the dominant sublattice slipped to a value below 0.5. There is a small error (of the order of 10 sites or less) in recording the domain size, introduced due to the domain wall being an extended object. Each disorder realization yields multiple domains, the typical size (and hence number per sample) being disorder and interaction strength dependent. While correlations in the location of domain walls in a single realization should exist, here we have ignored these and simply considered each domain as a statistically independent sample for the averaging procedure. Thus the disorder averaging is done over multiple realizations and domain sizes within each realization.

At the scale of 1000 sites, the finite size effects for all chains (random - monomer,dimer,trimer and quadrumer) are essentially negligible in the disordered regions (small domains). For example, for the random-monomer case, the Imry-Ma argument [4] holds and the chains are disordered at any non-zero disorder. This is seen in Fig. S1 (top panel) where we show average domain sizes for independent ensembles of 1000 and 2000 sites; the points for all disorder strengths lie essentially on top of each other and well within the errors due to the finite number of realizations used. The error bars refer to the standard deviation of the distribution of domain sizes.

The finite size effects are more pronounced in the regions

where an order to disorder transition occurs. This is primarily because of the contribution of domain sizes that exceed the length of the sample. (When no domain wall is found in the sample, we simply set the domain size to be the size of the sample. This introduces another bias). Such samples have finite weight in the ensemble and their contribution to the averaged domain size may be significant.

Fig. S1 (bottom panel) shows the difference between the $L = 1000$ and $L = 2000$ site ensembles of the random dimer model for disorder strengths where the first finite domains begin to form. For these transition regions, a precise estimate of the critical disorder strength would need a scaling theory, which remains to be developed for the form of correlated disorder considered here. However, a rough estimate of the transition point can still be made to within $\sim \pm 0.5t$.

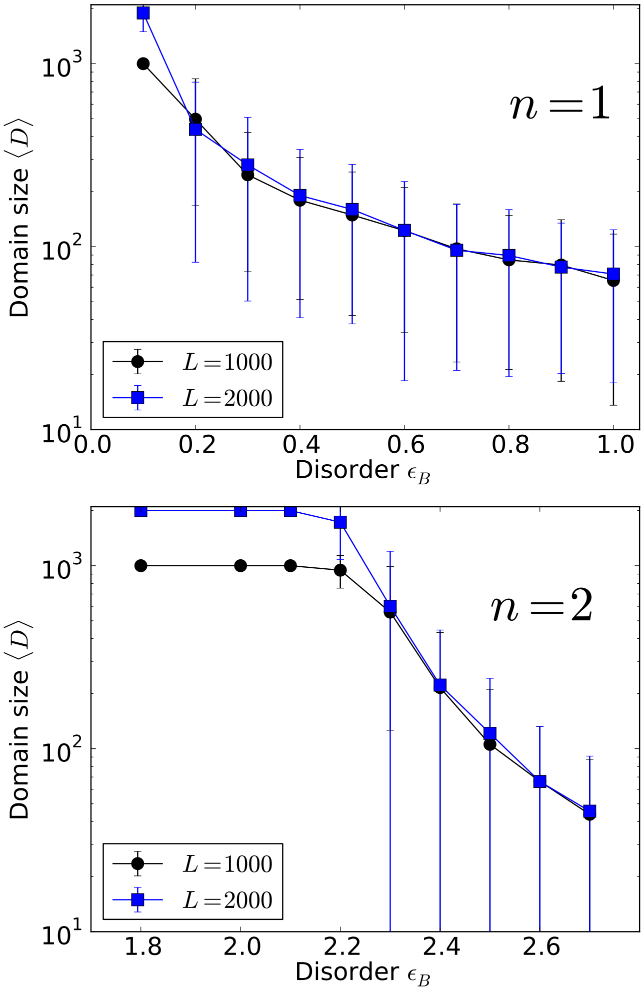


Figure S1. (Color online): Finite size dependence of domain size as a function of disorder strength (at $V/t = 5$) for the random monomer ($n = 1$, top panel) and dimer ($n = 2$, bottom panel) models using ensembles of 1000 and 2000 sites. Domains from each realization are treated as statistically independent samples in the averaging procedure. The error bars denote the standard deviation of the distribution ($\sigma$), and in most regions the error on the mean $\sigma/\sqrt{N_{samples}}$ is sufficiently small (of the order of size of the symbols). In the random dimer case, the spread in the distribution of domain wall sizes is large near the transition from ordered to disordered regions.

## II. RESULTS FOR SPECIAL INSTANCES OF DISORDERED CHAINS

In the text we described two special instances of disorder realizations that help understand the mechanisms for formation of domain walls (or phase slips). We discuss these in some more detail here.

### A. Single dimer in a clean chain

Consider a chain of even length $L$, with sites numbered from $1, 2...L$. Then place a dimer at the center of the chain i.e. at sites $i = L/2$ and $i = L/2 + 1$ set $\epsilon_i = \epsilon_B$, and for the rest of the chain $\epsilon_i = \epsilon_A = 0.0t$, except the left boundary which has the pinning field (described in the previous section). This chain is schematically depicted in Fig. S2 (top panel).

We monitor the CDW order in the sample as a function of $\epsilon_B$. We plot the density only on even sites, any transitions from high to low occupations in this plot indicate a domain wall or phase slip of the CDW order. As can be seen in Fig. S3, for small $\epsilon_B$ the CDW order persists; a small kink at the central sites is seen which is indicative of the slightly lower occupation of the $B$ site compared to the other high occupation $A$ sites participating in the CDW. At a critical $V$-dependent strength $\epsilon_B^*$, it is unfavorable for either of the $B$ sites to be (mostly) occupied. Once the occupation on this dimer is forced to be low, the $A$ sites on either end of it acquire high occupation numbers. Since these two $A$ sites are on opposite sublattices, the CDW on either side of the dimer is out of phase.

Despite this phase slip at the center of the sample, the pinning field at the left end eventually forces the CDW to change phase, gradually over the length of half the sample. (This effect can be minimized by making the strength of the pinning field smaller or the chain longer.)

### B. "Complement"-monomer chain

In the text we noted that the Imry-Ma argument is circumvented when the sublattice energies satisfy the condition,

$$\sum_{i \in 1} \epsilon_i - \sum_{j \in 2} \epsilon_j = 0 \tag{1}$$

where $\epsilon_{i(j)}$ refers to on-site energies on sites $i(j)$, and $1, 2$ is used to refer to sublattice indices. We emphasized that this condition must hold at all short and long length scales.

To provide an explicit example where this condition holds globally but not locally, we defined the "complement" chain. This is constructed by randomly generating a monomer chain

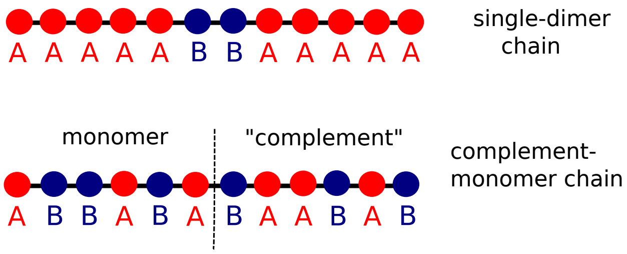


Figure S2. (Color online): Special one dimensional chains for demonstrating the mechanism of domain wall formation. Top: A single dimer of $B$ sites is embedded in an otherwise clean chain. Bottom: The complement-monomer chain is constructed by first generating an instance of a random monomer of length $L/2 = 6$ sites. Then its "complement" is defined as the chain obtained by replacing every $A$ by $B$ and $B$ by $A$. The monomer and complement are joined end to end to form the length $L = 12$ chain.

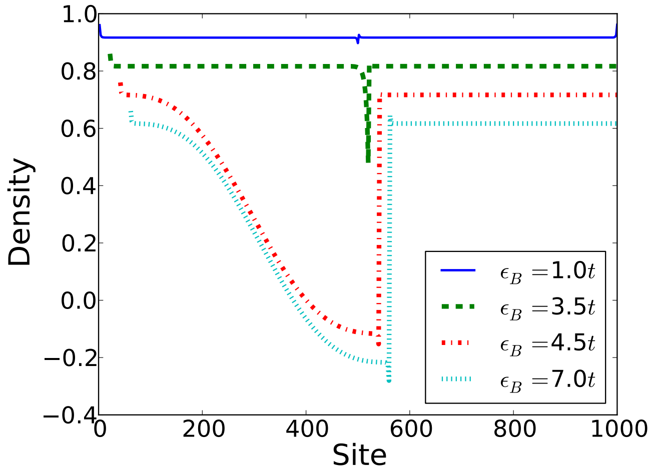


Figure S3. (Color online): Electron density on even sites for the chain with a single dimer embedded in the center, as a function of the disorder potential on the dimer $\epsilon_B$, at $V = 5.0t$. For clarity of the illustration, the density is shifted by amounts $(0.00, 0.10.0.20, 0.30)$ for $\epsilon_B/t = (1.0, 3.5, 4.5, 7)$ and correspondingly the location of the dimer (x axis) is shifted by amounts $(0, 20, 40, 60)$. For small disorder there is only a mild suppression of the electron density allowing the CDW to have the same phase on both sides of the chain. For larger disorder the CDW on either side of the dimer is out of phase. The pinning field at the left boundary (originally introduced to maintain one phase of the CDW in the clean chain) is responsible for the left-right asymmetry in the density. This field causes the CDW emerging from the left end of the dimer to change gradually to ensure that the left-most (boundary) site of the chain has low occupation.

of $L/2$ sites and its "complement", the latter obtained by replacing every $A$ type site by a $B$ type site and vice versa. Then these two segments are placed such that the end of the monomer connects to start of the complement, to form a $L$-site chain. A special instance of this chain is schematically depicted in Fig. S2 (bottom panel). We generated about 50 such correlated-disorder realizations and studied the formation of domains on varying the disorder strength $\epsilon_B$.

As is shown in Fig. S4, we find that for any non-zero disorder, the average domain size is finite (i.e. domain walls form), consistent with the Imry-Ma argument. While this is empirically evident for $V/t = 3$, there is a plateau-like feature for $V/t = 5$ and 7 at small disorder, similar to the one observed in the odd $n-$mer case. This is attributed primarily to the finite size of the lattice (1000 sites) which cannot support domains bigger than this scale. However, we note that based only on the data presented we can not completely rule out the possibility that the complement-monomer chain orders at a non-zero $\epsilon_B$ for some sufficiently large $V/t$.

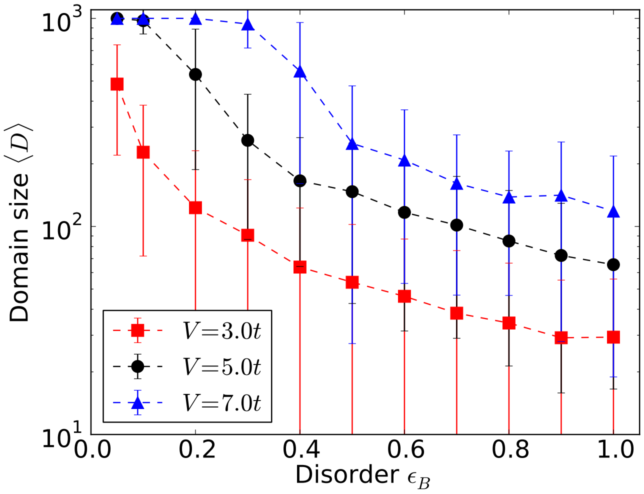


Figure S4. (Color online): Average of domain wall size ($\langle D \rangle$) versus disorder strength ($\epsilon_B$) for the "complement" monomer chain for various $V/t$. The error bars denote the standard deviation of the distribution ($\sigma$). The critical disorder for the occurrence of finite domain walls is consistent with zero, in agreement with the Imry-Ma argument.

[1] S. R. White, Phys. Rev. Lett. **69**, 2863 (1992).
[2] The ITensor library is a freely available code developed and maintained on http://itensor.org/index.html.
[3] B. Bauer, L. D. Carr, H. G. Evertz, A. Feiguin, J. Freire, S. Fuchs, L. Gamper, J. Gukelberger, E. Gull, S. Guertler, A. Hehn, R. Igarashi, S. V. Isakov, D. Koop, P. N. Ma, P. Mates, H. Matsuo, O. Parcollet, G. Pawlowski, J. D. Picon, L. Pollet, E. Santos, V. W. Scarola, U. Schollwöck, C. Silva, B. Surer, S. Todo, S. Trebst, M. Troyer, M. L. Wall, P. Werner, and S. Wessel, Journal of Statistical Mechanics: Theory and Experiment **2011**, P05001 (2011).
[4] Y. Imry and S.-k. Ma, Phys. Rev. Lett. **35**, 1399 (1975).
